# Supplementary material for: Submodular Maximization over Sliding Windows
Source: arXiv:1611.00129 source file (2016-11-01)
Supplement: Supplementary file 1 [file appendix.tex]

\section{Appendix}
